# Supplementary material for: Temporal Vectorization for Stencils
Source: arXiv:2010.04868 source file (2020-10-10)
Supplement: Supplementary file 1 [file stencil-appendix.tex]

\newpage
\appendix 
\onecolumn

Artifact Description

We now provide and describe our codes.
Our scheme is clear since it is based on a simple mathematical formulation. 
The following \texttt{kernel} can be any star or box stencil. 
\texttt{XSLOPE} and \texttt{YSLOPE} control the stencil size along each dimension.
In this work we only implement the non-periodic boundary condition.
However it's no hard to modify the code to handle stencils of periodic boundary conditions,
which is our ongoing work.
\texttt{level} controls the position of the two merged $(d+1)$-dimensional diamond, 
$\mathbb{B}_0 +\mathbb{B}_d$ from time tile of odd level to time tile of even level
and  $\mathbb{B}_d +\mathbb{B}_0$ from the opposite direction.
\texttt{xright[level]} is the right of the leftmost $\mathbb{B}_0$ block in time tile of that level.
\texttt{nb0[level]} is the number of $\mathbb{B}_0$ or  $\mathbb{B}_d$ blocks.

Here is the 1D code based on our tessellation scheme.

\begin{verbatim}
	int bx = atoi(argv[1]);
	int bt = atoi(argv[2]);
	int ix = bx + bx - 2 * bt * XSLOPE;
	int xright[2] = {bx + XSLOPE,  bx + XSLOPE - ix / 2};
	int nb0[2] = {(N + bx - (xright[0] - XSLOPE) - 1) / ix + 1,(N + bx - (xright[1] - XSLOPE) - 1) / ix + 1};
	
	int level = 0;
	int tt, n, t, x, xmin, xmax;
	
	for (tt = -bt; tt < T ;  tt += bt ){
		#pragma omp parallel for private(xmin,xmax,t,x)
		for(n = 0; n < nb0[level]; n++) {
			for(t = max(tt, 0) ; t < min( tt + 2 * bt,  T); t++){
				xmin = max(     XSLOPE, xright[level] - bx + n * ix + myabs(t+1, tt+bt) * XSLOPE);
				xmax = min( N + XSLOPE, xright[level]      + n * ix - myabs(t+1, tt+bt) * XSLOPE);
				#pragma ivdep
				for(x = xmin; x < xmax; x++){
					update(t, x);}}}
		level = 1 - level;}
\end{verbatim}

Here is the 2D code based on our tessellation scheme.

\begin{verbatim}
	int Bx = atoi(argv[1]);
	int By = atoi(argv[2]);
	int bt = atoi(argv[3]);
	int bx = Bx-2*(bt*XSLOPE);
	int by = By-2*(bt*YSLOPE);
	int ix=Bx+bx;
	int iy=By+by;
	int xnb0=ceild(NX,ix);
	int ynb0=ceild(NY,iy);
	int xnb11=ceild(NX-ix/2+1,ix) +1;
	int ynb11= ynb0;
	int xnb12= xnb0;
	int ynb12=1+ceild(NY-iy/2+1,iy);
	int xnb2=max(xnb11,xnb0);
	int ynb2=max(ynb12,ynb0);
	int nb1[2] = {xnb12 * ynb12, xnb11 * ynb11};
	int nb02[2] = {xnb2 * ynb2, xnb0 * ynb0};// B_0 and B_2 are merged to a 3-d diamond
	int xnb1[2] = {xnb12, xnb11};
	int xnb02[2] = {xnb2, xnb0};
	int xleft02[2] = {XSLOPE-bx, XSLOPE+(Bx-bx)/2};
	int ybottom02[2] = {YSLOPE-by, YSLOPE+(By-by)/2};
	int xleft11[2] = {XSLOPE+(Bx-bx)/2, XSLOPE - bx};
	int ybottom11[2] = {YSLOPE-(By+by)/2, YSLOPE};
	int xleft12[2] = {XSLOPE-(Bx+bx)/2, XSLOPE};
	int ybottom12[2] = {YSLOPE+(By-by)/2, YSLOPE-by};

	int level = 1;
	int tt, n, t, x, y, xmin, xmax, ymin, ymax;
	for(tt = -bt; tt < T; tt += bt){		
		#pragma omp parallel for private(xmin,xmax,ymin,ymax,t,x,y)
		for(n = 0; n < nb02[level]; n++){
			for(t = max(tt,0); t < min( tt + 2*bt,  T); t++){ 
				xmin = max(     XSLOPE,   xleft02[level] + (n%xnb02[level]) * ix      - bt*XSLOPE + abs(t+1, tt+bt) * XSLOPE);
				xmax = min(NX + XSLOPE,   xleft02[level] + (n%xnb02[level]) * ix + bx + bt*XSLOPE - abs(t+1, tt+bt) * XSLOPE);
				ymin = max(     YSLOPE, ybottom02[level] + (n/xnb02[level]) * iy      - bt*YSLOPE + abs(t+1, tt+bt) * YSLOPE);
				ymax = min(NY + YSLOPE, ybottom02[level] + (n/xnb02[level]) * iy + by + bt*YSLOPE - abs(t+1, tt+bt) * YSLOPE);
				for(x = xmin; x < xmax; x++) {
					#pragma ivdep 
					for(y = ymin; y < ymax; y++){
						update(t, x, y); }}}}
		#pragma omp parallel for private(xmin,xmax,ymin,ymax,t,x,y)
		for(n = 0; n < nb1[0] + nb1[1]; n++){
			for(t = tt+bt ; t < min( tt + 2*bt,  T); t++) {
				if(n<nb1[level]){
					xmin = max(     XSLOPE,   xleft11[level] +                (n%xnb1[level]) * ix      - (t+1-tt-bt) * XSLOPE);
					xmax = min(NX + XSLOPE,   xleft11[level] +                (n%xnb1[level]) * ix + bx + (t+1-tt-bt) * XSLOPE);
					ymin = max(     YSLOPE, ybottom11[level] +                (n/xnb1[level]) * iy      + (t+1-tt-bt) * YSLOPE);
					ymax = min(NY + YSLOPE, ybottom11[level] +                (n/xnb1[level]) * iy + By - (t+1-tt-bt) * YSLOPE); }
				else{
					xmin = max(     XSLOPE,   xleft12[level] + ((n-nb1[level])%xnb1[1-level]) * ix      + (t+1-tt-bt) * XSLOPE);
					xmax = min(NX + XSLOPE,   xleft12[level] + ((n-nb1[level])%xnb1[1-level]) * ix + Bx - (t+1-tt-bt) * XSLOPE);
					ymin = max(     YSLOPE, ybottom12[level] + ((n-nb1[level])/xnb1[1-level]) * iy      - (t+1-tt-bt) * YSLOPE);
					ymax = min(NY + YSLOPE, ybottom12[level] + ((n-nb1[level])/xnb1[1-level]) * iy + by + (t+1-tt-bt) * YSLOPE); }
				for(x = xmin; x < xmax; x++) {
					#pragma ivdep
					for(y = ymin; y < ymax; y++){
						update(t, x, y); }}}}
			level = 1 - level;}
\end{verbatim}
